# Supplementary material for: Multi-threshold time series analysis enables characterization of variable renewable energy droughts in Europe
Source: arXiv:2410.00244 source file (2026-01-29)
Supplement: Supplementary file 1 [file Figure_SI12.pdf]

Germany

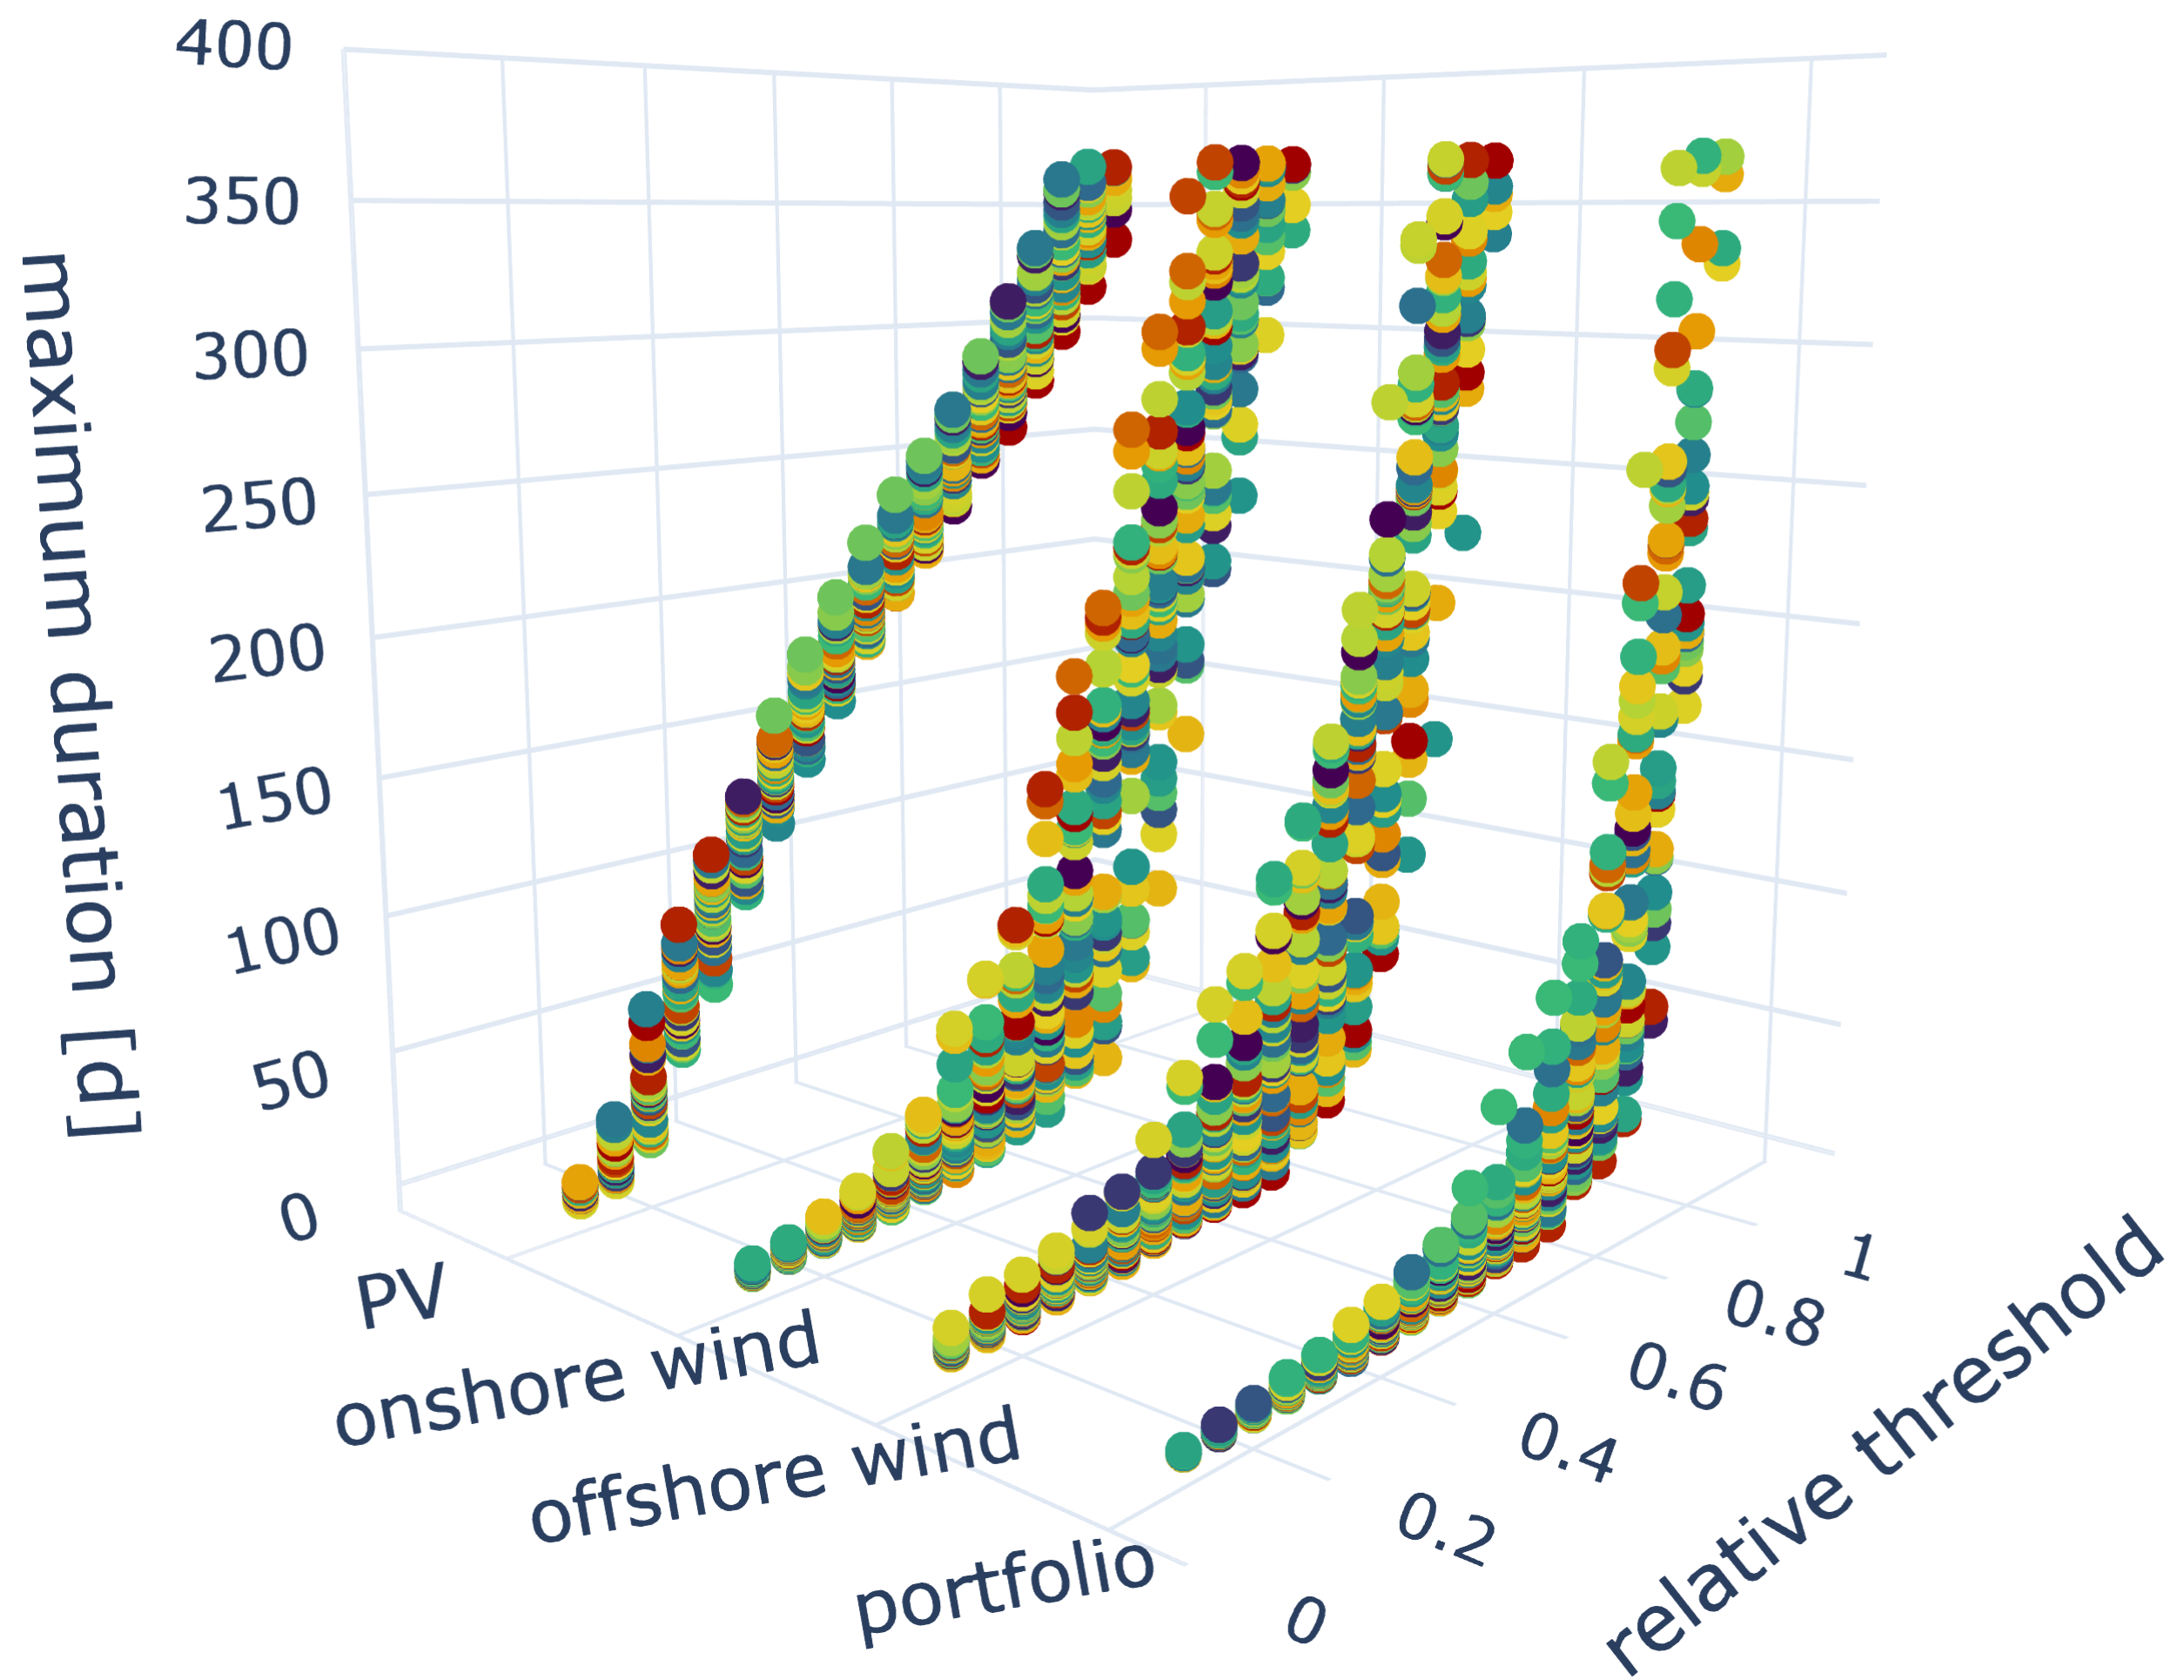

Spain

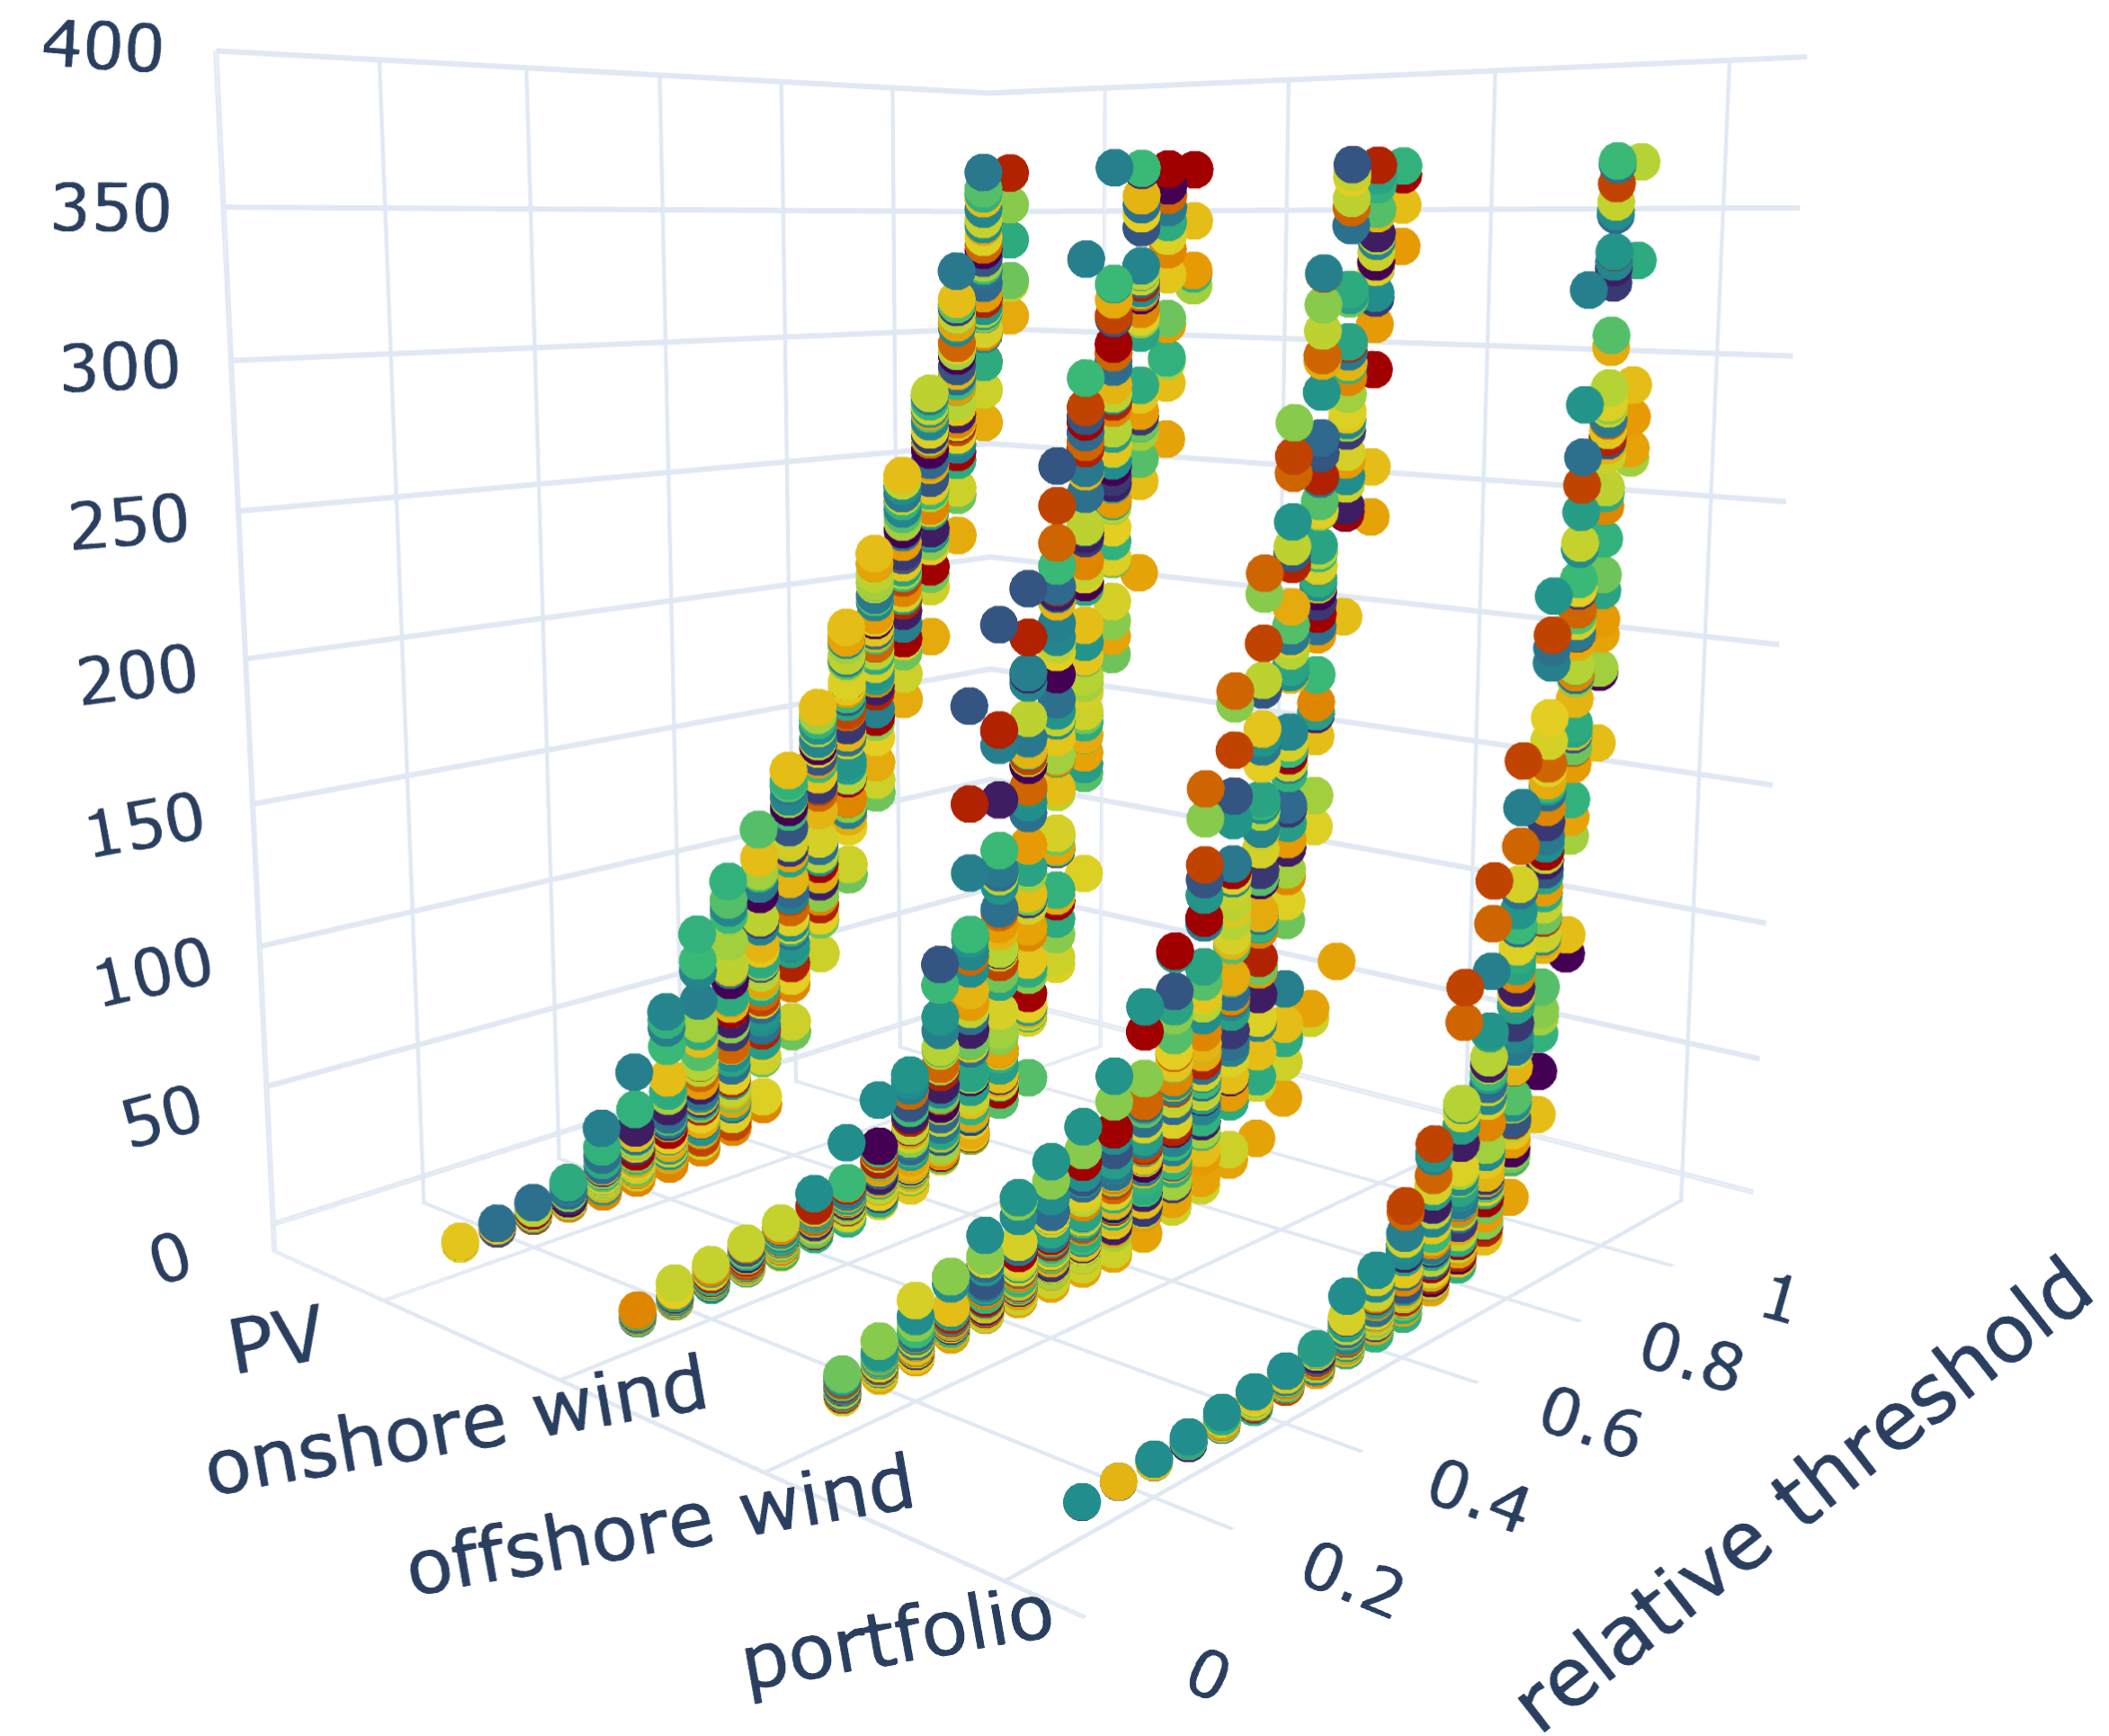

European copperplate

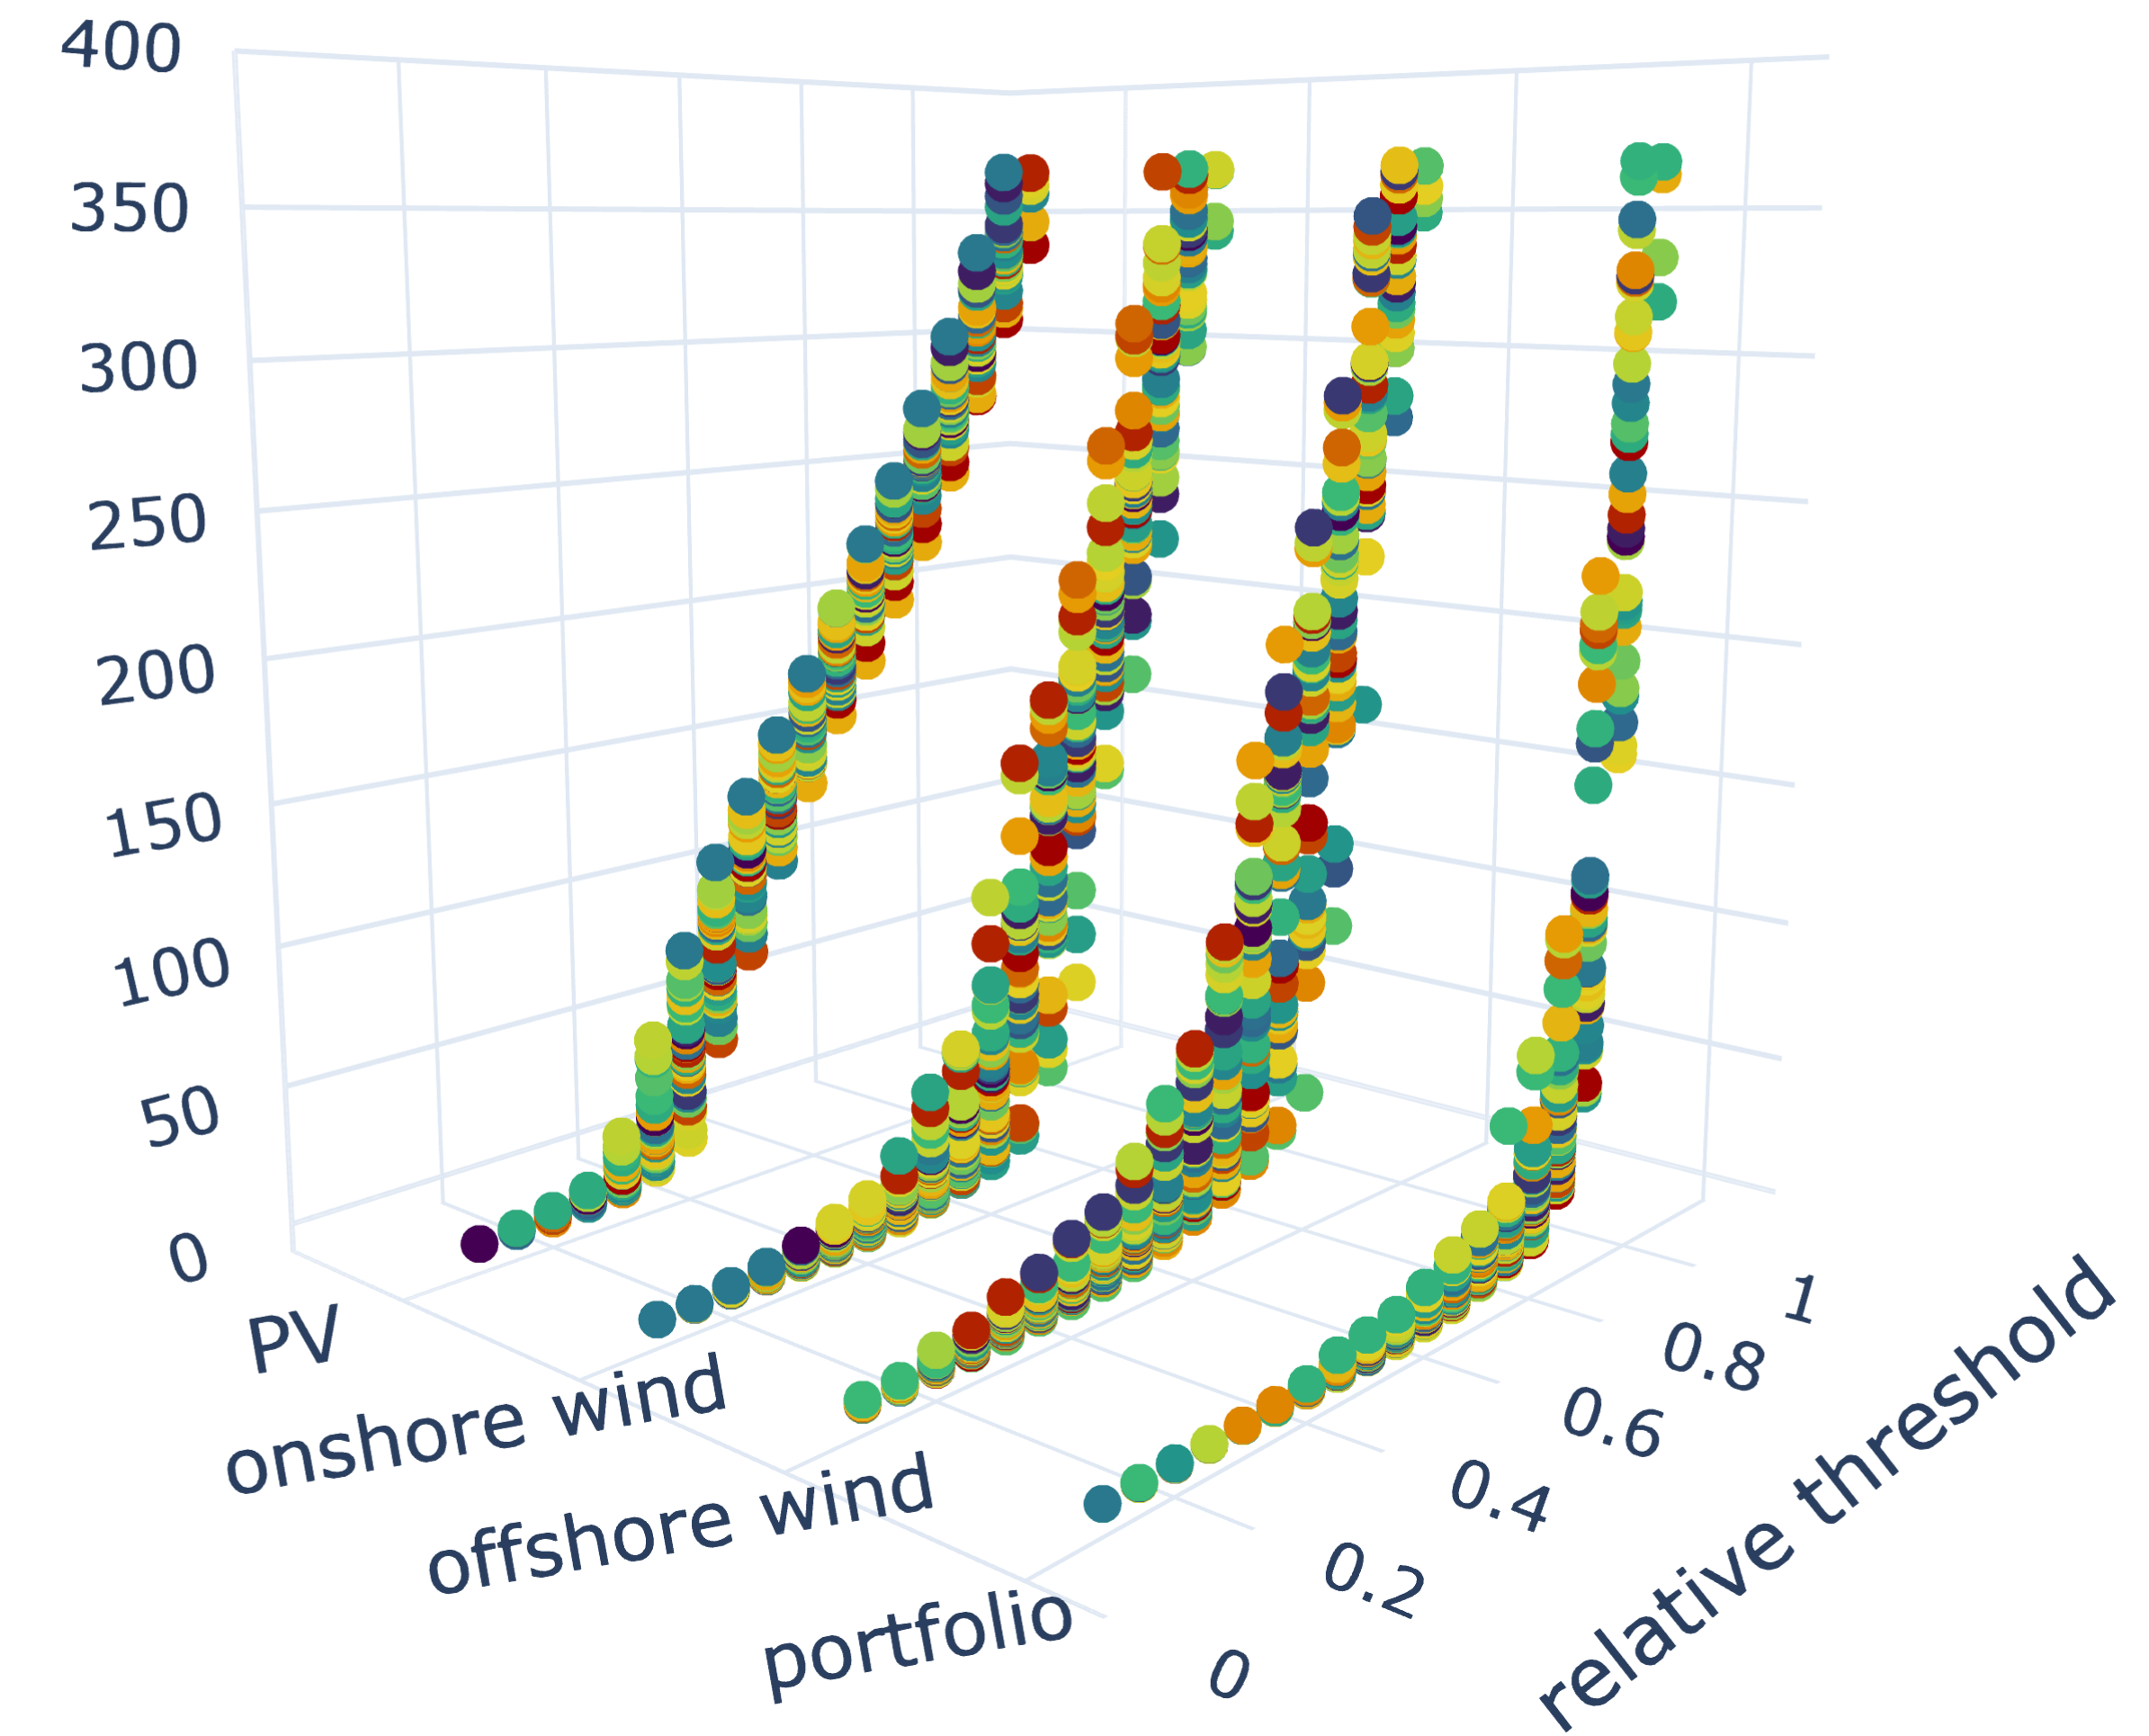

1985

1990

1995

2000

2005

2010

2015
